# Supplementary material for: An Empirical Study of the Impact of Federated Learning on Machine Learning Model Accuracy
Source: arXiv:2503.20768 source file (2025-03-27)
Supplement: Supplementary file 1 [file appendix.tex]

%\begin{appendix}
%Appendix here.

%\end{appendix}
